# Supplementary material for: Assessing the Reproducibility of Machine-learning-based Biomarker Discovery in Parkinson's Disease
Source: arXiv:2304.03239 source file (2023-04-06)
Supplement: Supplementary file 1 [file SupplementaryFile.pdf]

# Supplementary Material

We selected the SNPs identified by at least two datasets or two approaches and listed their associated phenotype in Tables 1, 2, 3, 4, 5, 6 ,and 7 (we have several small tables because it is difficult to fit all this information into one single table). The third column lists the approaches and datasets were the corresponding SNP was in the list of frequent SNPs. Some of these SNPs were linked to other diseases, however the diseases highlighted were linked to PD indirectly.

We identified four SNP IDs (11248060, rs239748, rs999473, and rs231398) that have a direct link with PD (see table 6). Additional research demonstrates that 50 identified SNP IDs (rs13006682, rs1037100, rs1367445, rs2827784, rs4409785, rs11727767, rs2551043, rs7039377, rs4984406, rs1420956, rs2070762, rs4794665, rs6088520, rs2240308, rs2298632, rs3892715, rs4077636, rs7152906, rs1950829, rs1801274, rs12490036, rs12643013, rs6749972, rs1801274, rs1919309, rs2284178, rs901273, rs10894032, rs4300072, rs7554436, rs7646765, rs130423, rs12659814, rs252139, rs194933, rs934178, rs1870676, rs6590810, rs1007415, rs385893, rs11076194, rs4771493, rs4886755, rs799160, rs7026582, rs706779, rs799160, rs9303277, rs9409664, and rs10117) are indirectly associated with PD. These indirectly associated SNPs can be further investigated as potential biomarkers for PD.

Direct association means that current literature directly links a SNP with PD; while an indirect link means that current literature suggests the involvement of a SNP in a disease other than PD but this other disease co-occurs with PD in a significant number of PD patients.

| SNPs ID | Phenotypes | Datasets / Approaches | Literature linking phenotype to PD |
|---|---|---|---|
| rs13006682<br>rs1037100 | PR interval (The time between atrial depolarization and ventricular depolarization) | Approach 0 (NINDS1 and NINDS2)<br>Approach 4 (Autopsy and NINDS1)<br>NINDS1 (Approach 2 and Approach 3)<br>NINDS1 (Approach 2 and Approach 4)<br>NINDS1 (Approach 3 and Approach 4) | [1] |
| rs1367445 | Osteoporosis Lumbar Spine BMD(bone density) | Approach 0 (NINDS1 and NINDS2) | [2][3][4][5] |
| rs2827784 | C-reactive protein | Approach 0 (NINDS1 and NINDS2) | [6][7] |
| rs4409785 | Rheumatoid arthritis | Approach 0 (NINDS1 and NINDS2) | [8][9][10][11] |
| | Vitiligo | Approach 0 (NINDS1 and NINDS2) | [12] |
| | Sex hormone-binding globulin levels | Approach 0 (NINDS1 and NINDS2) | [13][14] |
| | Myasthenia gravis | Approach 0 (NINDS1 and NINDS2) | [15] |
| | Multiple sclerosis and Low Density Lipoprotein (LDL) levels | Approach 0 (NINDS1 and NINDS2) | [16][17] |
| | Multiple sclerosis | Approach 0 (NINDS1 and NINDS2) | [18] |
| | Medication use thyroid preparations | Approach 0 (NINDS1 and NINDS2) | [19] |
| | Hypothyroidism, | Approach 0 (NINDS1 and NINDS2) | [20],[21] |
| | Graves disease | Approach 0 (NINDS1 and NINDS2) | [22] |
| | Eosinophil counts | Approach 0 (NINDS1 and NINDS2) | [23][24] |
| | Autoimmune traits | Approach 0 (NINDS1 and NINDS2) | [25][26] |
| | Autoimmune thyroid diseases (Graves'disease or Hashimoto's thyroiditis) | Approach 0 (NINDS1 and NINDS2) | [27][28] |

Table 1: SNPs in association with phenotypes - 1

| SNPs ID | Phenotypes | Datasets / Approaches | Literature linking phenotype to PD |
|---|---|---|---|
| rs11727767<br>rs2551043<br>rs7039377<br>rs4984406<br>rs1420956 | Obesity-related traits | Approach 1 (Autopsy and NINDS1)<br>Approach 1 (NINDS1 and Tier1)<br>Approach 2 (Autopsy and NINDS1)<br>Approach 4 (Autopsy and NINDS1)<br>Autopsy (Approach 1 and Approach 2)<br>Autopsy (Approach 2 and Approach 4)<br>NINDS1 (Approach 1 and Approach 2)<br>NINDS1 (Approach 1 and Approach 2)<br>NINDS1 (Approach 3 and Approach 4) | [29][30][31][32] |
| rs2070762<br>rs4794665<br>rs6088520 | Height | Approach 1 (Autopsy and NINDS1)<br>Approach 2 (Autopsy and NINDS1)<br>Autopsy (Approach 1 and Approach 2)<br>Autopsy (Approach 3 and Approach 4)<br>NINDS1 (Approach 1 and Approach 2)<br>NINDS1 (Approach 1 and Approach 3)<br>NINDS1 (Approach 1 and Approach 4)<br>NINDS1 (Approach 2 and Approach 3)<br>NINDS1 (Approach 2 and Approach 4)<br>NINDS1 (Approach 3 and Approach 4)<br>Tier1 (Approach 3 and Approach 4) | [33][34][35] |
| rs2240308 | Oligodontia-colorectal cancer syndrome | Approach 1 (Autopsy and NINDS1) | [36] |

Table 2: SNPs in association with phenotypes - 2

| SNPs ID | Phenotypes | Datasets / Approaches | Literature linking phenotype to PD |
|---|---|---|---|
| rs2298632 | QT interval (The time it takes for the electrical system to fire an impulse through the ventricles and then recharge) | Approach 1 (Autopsy and NINDS1) | [37][38] |
| | High Density Lipoprotein (HDL) cholesterol | Approach 1 (Autopsy and NINDS1)<br>Approach 2 (Autopsy and NINDS1)<br>Autopsy (Approach 1 and Approach 2)<br>NINDS1 (Approach 1 and Approach 2) | [39][40] |
| | Electrocardiographic traits multivariate | Approach 1 (Autopsy and NINDS1)<br>Approach 2 (Autopsy and NINDS1)<br>Autopsy (Approach 1 and Approach 2) | [41] |
| rs3892715 | Attention Deficit Hyperactivity Disorder (ADHD) | Approach 1 (Autopsy and NINDS1)<br>NINDS1 (Approach 1 and Approach 3)<br>NINDS1 (Approach 1 and Approach 4)<br>NINDS1 (Approach 3 and Approach 4) | [42][43][44] |
| rs4077636 | Lung function FEV1 (The amount of air exhaled may be measured during the first)/Forced vital capacity (FVC) | Approach 1 (Autopsy and NINDS1)<br>Approach 1 (Autopsy and Tier1)<br>Approach 1 (NINDS1 and Tier1)<br>Approach 2 (Autopsy and NINDS1)<br>Approach 2 (Autopsy and Tier1)<br>Approach 2 (NINDS1 and Tier1)<br>Autopsy (Approach 1 and Approach 2)<br>NINDS1 (Approach 1 and Approach 2)<br>NINDS1 (Approach 3 and Approach 4)<br>Tier1 (Approach 1 and Approach 2) | [45] |

Table 3: SNPs in association with phenotypes - 3

| SNPs ID | Phenotypes | Datasets / Approaches | Literature linking phenotype to PD |
|---|---|---|---|
| rs7152906<br>rs1950829 | Major depressive disorder Multi Trait Analysis of GWAS (MTAG) | Approach 1 (Autopsy and NINDS1)<br>Approach 2 (Autopsy and NINDS1)<br>Approach 2 (NINDS1 and Tier1)<br>Autopsy (Approach 1 and Approach 2)<br>Autopsy (Approach 1 and Approach 3)<br>Autopsy (Approach 1 and Approach 4)<br>Autopsy (Approach 2 and Approach 3)<br>Autopsy (Approach 2 and Approach 4)<br>Autopsy (Approach 3 and Approach 4)<br>NINDS1 (Approach 1 and Approach 2)<br>Tier1 (Approach 1 and Approach 2) | [46][47][48] |
| rs1801274 | Programmed Death Ligand 1 (PDL-1) on cluster of differentiation 14 (CD14+), cluster of differentiation 14 (CD16+) monocyte | Approach 1 (NINDS1 and Tier1)<br>Approach 2 (NINDS1 and Tier1)<br>NINDS1 (Approach 1 and Approach 2)<br>Tier1 (Approach 1 and Approach 2) | [49][50] |
| | Inflammatory bowel disease | Approach 1 (NINDS1 and Tier1)<br>NINDS1 (Approach 1 and Approach 2)<br>Tier1 (Approach 1 and Approach 2) | [51][52][53] |
| rs12490036 | Mean corpuscular hemoglobin concentration | Approach 2 (Autopsy and NINDS1)<br>Autopsy (Approach 2 and Approach 4) | [54][55][56][57] |
| rs12643013 | Iron | Approach 2 (Autopsy and NINDS1) | [58][59] |
| rs6749972 | Smoking initiation (ever regular vs never regular) (MTAG) | Approach 2 (Autopsy and NINDS1) | [60][61] |
| rs1801274 | Ankylosing spondylitis | Approach 2 (NINDS1 and Tier1)<br>NINDS1 (Approach 1 and Approach 2)<br>Tier1 (Approach 1 and Approach 2) | [62] |
| rs1919309 | Apolipoprotein A1 levels | Approach 3 (Autopsy and NINDS1)<br>NINDS1 (Approach 3 and Approach 4) | [62][63] |

Table 4: SNPs in association with phenotypes - 4

| SNPs ID | Phenotypes | Datasets / Approaches | Literature linking phenotype to PD |
|---|---|---|---|
| rs2284178 | Behcet Syndrome | Approach 3 (Autopsy and NINDS1)<br>Approach 4 (Autopsy and NINDS1)<br>Autopsy (Approach 3 and Approach 4)<br>NINDS1 (Approach 3 and Approach 4) | [64] |
| rs901273<br>rs10894032<br>rs4300072<br>rs7554436<br>rs7646765 | Stroke | Approach 3 (Autopsy and NINDS1)<br>Approach 4 (Autopsy and NINDS1)<br>Autopsy (Approach 3 and Approach 4)<br>NINDS1 (Approach 3 and Approach 4) | [65][66] |
| rs130423 | Glucose | Approach 3 (Autopsy and NINDS2)<br>Approach 4 (Autopsy and NINDS1)<br>Approach 4 (Autopsy and NINDS2)<br>Approach 4 (NINDS1 and NINDS2)<br>Autopsy (Approach 3 and Approach 4)<br>NINDS2 (Approach 3 and Approach 4) | [67][68] |
| rs12659814 | Creatinine | Approach 3 (NINDS1 and NINDS2) | [69][70] |
| rs252139 | Amyotrophic lateral sclerosis | Approach 3 (NINDS1 and NINDS2) | [71] |
| rs194933 | Heart Rate | Approach 4 (Autopsy and NINDS1)<br>NINDS1 (Approach 3 and Approach 4) | [72][73] |

Table 5: SNPs in association with phenotypes - 5

| SNPs ID | Phenotypes | Datasets / Approaches | Literature linking phenotype to PD |
|---|---|---|---|
| rs934178 | Red cell distribution width | Autopsy (Approach 1 and Approach 2)<br>Autopsy (Approach 2 and Approach 3)<br>Autopsy (Approach 2 and Approach 4)<br>Autopsy (Approach 3 and Approach 4) | [74] |
| rs1870676 | Intelligence | Autopsy (Approach 3 and Approach 4) | [75] |
| rs6590810 | Hair color | NINDS1 (Approach 1 and Approach 2) | [76] |
| rs1007415<br>rs385893 | Platelet Count | NINDS1 (Approach 3 and Approach 4) | [77] |
| rs11076194 | Heel bone mineral density | NINDS1 (Approach 3 and Approach 4) | [78][4] |
| rs4771493 | Numerical cognitive ability | NINDS1 (Approach 3 and Approach 4) | [79] |
| rs11248060<br>rs239748<br>rs999473<br>rs2313982 | Parkinson's disease (PD) | NINDS1 (Approach 3 and Approach 4)<br>Tier1 (Approach 3 and Approach 4) | Direct link with PD |
| rs4886755<br>rs799160 | Urate levels | NINDS1 (Approach 3 and Approach 4)<br>Tier1 (Approach 2 and Approach 3) | [80][81] |
| | Hemoglobin | NINDS1 (Approach 3 and Approach 4) | [82][83] |
| rs7026582 | Lipids | NINDS1 (Approach 3 and Approach 4) | [84] |

Table 6: SNPs in association with phenotypes - 6

| SNPs ID | Phenotypes | Datasets / Approaches | Literature linking phenotype to PD |
|---|---|---|---|
| rs706779 | Vitiligo | NINDS1 (Approach 3 and Approach 4) | [85] |
| | Type 1 diabetes | NINDS1 (Approach 3 and Approach 4) | [86][87] |
| rs799160 | Triglyceride levels | Tier1 (Approach 2 and Approach 3) | [88] |
| rs9303277 | Primary biliary cholangitis | Tier1 (Approach 2 and Approach 3) | [89][90] |
| rs9409664 | Inflammation | Tier1 (Approach 2 and Approach 3)<br>Tier1 (Approach 2 and Approach 4)<br>Tier1 (Approach 3 and Approach 4) | [91][92] |
| rs10117 | Even-plus syndrome | Tier1 (Approach 3 and Approach 4) | [93] |

Table 7: SNPs in association with phenotypes - 7

## References


[1] H. Mochizuki, Y. Ebihara, Y. Ugawa, N. Ishii, A. Taniguchi, S. Nagamachi, K. Shiomi, and M. Nakazato, "PR prolongation and cardiac 123I-MIBG uptake reduction in Parkinson's disease," *European Neurology*, vol. 74, no. 1-2, pp. 107–111, 2015.

[2] C. A. Figueroa and C. J. Rosen, "Parkinson's disease and osteoporosis: basic and clinical implications," *Expert Review of Endocrinology & Metabolism*, vol. 15, no. 3, pp. 185–193, 2020.

[3] L. M. Raglione, S. Sorbi, and B. Nacmias, "Osteoporosis and Parkinson's disease," *Clinical Cases in Mineral and Bone Metabolism*, vol. 8, no. 3, p. 16, 2011.

[4] H. Gao, X. Wei, J. Liao, R. Wang, J. Xu, X. Liu, X. Pan, Z. Li, Z. Li, Y. Xia *et al.*, "Lower bone mineral density in patients with Parkinson's disease: a cross-sectional study from Chinese Mainland," *Frontiers in Aging Neuroscience*, vol. 7, p. 203, 2015.

[5] F. Van Den Bos, A. D. Speelman, M. Samson, M. Munneke, B. R. Bloem, and H. J. Verhaar, "Parkinson's disease and osteoporosis," *Age and Ageing*, vol. 42, no. 2, pp. 156–162, 2013.

[6] X. Qiu, Y. Xiao, J. Wu, L. Gan, Y. Huang, and J. Wang, "C-reactive protein and risk of Parkinson's disease: a systematic review and meta-analysis," *Frontiers in Neurology*, vol. 10, p. 384, 2019.

[7] P. Lyra, J. Botelho, V. Machado, S. Rota, R. Walker, J. Staunton, L. Proença, K. R. Chaudhuri, and J. J. Mendes, "Self-reported periodontitis and C-reactive protein in Parkinson's disease: a cross-sectional study of two American cohorts," *npj Parkinson's Disease*, vol. 8, no. 1, pp. 1–6, 2022.

[8] T. Kogure, T. Tatsumi, Y. Kaneko, and K. Okamoto, "Rheumatoid arthritis accompanied by Parkinson's disease," *JCR: Journal of Clinical Rheumatology*, vol. 14, no. 3, pp. 192–193, 2008.

[9] D. Li, X. Hong, and T. Chen, "Association between rheumatoid arthritis and risk of Parkinson's disease: A meta-analysis and systematic review," *Frontiers in Neurology*, vol. 13, 2022.

[10] C. Li, R. Ou, and H. Shang, "Rheumatoid arthritis decreases risk for Parkinson's disease: a mendelian randomization study," *npj Parkinson's Disease*, vol. 7, no. 1, pp. 1–5, 2021.

[11] J. Bacelis, M. Compagno, S. George, J. A. Pospisilik, P. Brundin, Å. T. Naluai, and L. Brundin, "Decreased risk of Parkinson's disease after rheumatoid arthritis diagnosis: a nested case-control study with matched cases and controls," *Journal of Parkinson's Disease*, vol. 11, no. 2, pp. 821–832, 2021.

[12] B. Bellei, A. Pitisci, M. Ottaviani, M. Ludovici, C. Cota, F. Luzi, M. L. Dell'Anna, and M. Picardo, "Vitiligo: a possible model of degenerative diseases," *PlOS One*, vol. 8, no. 3, p. e59782, 2013.

[13] M. Nitkowska, R. Tomasiuk, M. Czyżyk, and A. Friedman, "Prolactin and sex hormones levels in males with Parkinson's disease," *Acta Neurologica Scandinavica*, vol. 131, no. 6, pp. 411–416, 2015.

[14] C. Kusters, K. Paul, A. D. Folle, A. Keener, J. Bronstein, L. Bertram, J. Hansen, S. Horvath, J. Sinsheimer, C. Lill *et al.*, "SHBG, and possibly testosterone, are associated with the risk for Parkinson's disease among women: a Mendelian randomization approach," in *Movement Disorders*, vol. 36. Wiley 111 River St, Hoboken 07030-5774, Nj USA, 2021, pp. S313–S313.

[15] I. Odajiu, E. I. Davidescu, C. Mitu, and B. O. Popescu, "Patients with Parkinson's disease and myasthenia gravis—a report of three new cases and review of the literature," *Medicina*, vol. 56, no. 1, p. 5, 2019.

[16] A. Witoelar, I. E. Jansen, Y. Wang, R. S. Desikan, J. R. Gibbs, C. Blauwendraat, W. K. Thompson, D. G. Hernandez, S. Djurovic, A. J. Schork *et al.*, "Genome-wide pleiotropy between Parkinson's disease and autoimmune diseases," *JAMA Neurology*, vol. 74, no. 7, pp. 780–792, 2017.

[17] X. Zhang, A. M. Lucas, Y. Veturi, T. G. Drivas, W. P. Bone, A. Verma, W. K. Chung, D. Crosslin, J. C. Denny, S. Hebbring *et al.*, "Large-scale genomic analyses reveal insights into pleiotropy across circulatory system diseases and nervous system disorders," *Nature Communications*, vol. 13, no. 1, pp. 1–12, 2022.

[18] V. Shaygannejad, M. Shirmardi, L. Dehghani, and H. Maghzi, "Co-occurrence of multiple sclerosis and Parkinson's disease," *Advanced Biomedical Research*, vol. 5, 2016.

[19] T. D. Wingert and J. M. Hershman, "Sinemet® and thyroid function in Parkinson's disease," *Neurology*, vol. 29, no. 7, pp. 1073–1073, 1979.

[20] S.-F. Chen, Y.-C. Yang, C.-Y. Hsu, and Y.-C. Shen, "Risk of Parkinson's disease in patients with hypothyroidism: A nationwide population-based cohort study," *Parkinsonism & Related Disorders*, vol. 74, pp. 28–32, 2020.

[21] J. Garcia-Moreno and J. Chacon, "Hypothyroidism concealed by Parkinson's disease," *Revista de Neurologia*, vol. 35, no. 8, pp. 741–742, 2002.

[22] Y. Y. Cho, B. Kim, D. W. Shin, J. Youn, J. O. Mok, C.-H. Kim, S. W. Kim, J. H. Chung, K. Han, and T. H. Kim, "Graves' disease and the risk of Parkinson's disease: a Korean population-based study," *Brain Communications*, vol. 4, no. 1, p. fcac014, 2022.

[23] M. P. Jensen, B. M. Jacobs, R. Dobson, S. Bandres-Ciga, C. Blauwendraat, A. Schrag, A. J. Noyce, and I. Parkinson's Disease Genomics Consortium (IPDGC), "Lower lymphocyte count is associated with increased risk of Parkinson's disease," *Annals of Neurology*, vol. 89, no. 4, pp. 803–812, 2021.

[24] G.-T. Liu, C.-S. Hwang, C.-H. Hsieh, C.-H. Lu, S. L.-Y. Chang, J.-C. Lee, C.-F. Huang, and H.-T. Chang, "Eosinophil-derived neurotoxin is elevated in patients with amyotrophic lateral sclerosis," *Mediators of Inflammation*, vol. 2013, 2013.

[25] K. Rugbjerg, S. Friis, B. Ritz, E. Schernhammer, L. Korbo, and J. Olsen, "Autoimmune disease and risk for Parkinson's disease: a population-based case-control study," *Neurology*, vol. 73, no. 18, pp. 1462–1468, 2009.

[26] F. Garretti, D. Agalliu, C. S. Lindestam Arlehamn, A. Sette, and D. Sulzer, "Autoimmunity in Parkinson's disease: the role of $\alpha$-synuclein-specific T cells," *Frontiers in Immunology*, vol. 10, p. 303, 2019.

[27] N. Charoenngam, T. Rittiphairoj, B. Ponvilawan, and K. Prasongdee, "Thyroid Dysfunction and risk of Parkinson's disease: A Systematic Review and Meta-Analysis," *Frontiers in Endocrinology*, vol. 13, 2022.

[28] U. Bonuccelli, C. D'Avino, N. Caraccio, P. Del Guerra, A. Casolaro, N. Pavese, P. Del Dotto, and F. Monzani, "Thyroid function and autoimmunity in Parkinson's disease: a study of 101 patients," *Parkinsonism & Related Disorders*, vol. 5, no. 1-2, pp. 49–53, 1999.

[29] N. Palacios, X. Gao, M. L. McCullough, E. J. Jacobs, A. V. Patel, T. Mayo, M. A. Schwarzschild, and A. Ascherio, "Obesity, diabetes, and risk of Parkinson's disease," *Movement Disorders*, vol. 26, no. 12, pp. 2253–2259, 2011.

[30] J. Chen, Z. Guan, L. Wang, G. Song, B. Ma, and Y. Wang, "Meta-analysis: overweight, obesity, and Parkinson's disease," *International Journal of Endocrinology*, vol. 2014, 2014.

[31] Y.-L. Wang, Y.-T. Wang, J.-F. Li, Y.-Z. Zhang, H.-L. Yin, and B. Han, "Body mass index and risk of Parkinson's disease: a dose-response meta-analysis of prospective studies," *PlOS One*, vol. 10, no. 6, p. e0131778, 2015.

[32] K.-Y. Park, G. E. Nam, K. Han, H.-K. Park, and H.-S. Hwang, "Waist circumference and risk of Parkinson's disease," *npj Parkinson's Disease*, vol. 8, no. 1, pp. 1–8, 2022.

[33] P. Ragonese, M. D'Amelio, G. Callari, F. Aiello, L. Morgante, and G. Savettieri, "Height as a potential indicator of early life events predicting Parkinson's disease: A case-control study," *Movement Disorders: Official Journal of the Movement Disorder Society*, vol. 22, no. 15, pp. 2263–2267, 2007.

[34] U. M. Fietzek, F. E. Schroeteler, L. Hahn, K. Ziegler, and A. O. Ceballos-Baumann, "Body height loss characterizes camptocormia in Parkinson's disease," *Journal of Neural Transmission*, vol. 125, no. 10, pp. 1473–1480, 2018.

[35] L. Saari, E. A. Backman, P. Wahlsten, M. Gardberg, and V. Kaasinen, "Height and nigral neuron density in Parkinson's disease," *BMC Neurology*, vol. 22, no. 1, pp. 1–6, 2022.

[36] H. Fang, Y. Du, S. Pan, M. Zhong, and J. Tang, "Patients with Parkinson's disease predict a lower incidence of colorectal cancer," *BMC Geriatrics*, vol. 21, no. 1, pp. 1–8, 2021.

[37] H. Oka, S. Mochio, H. Sato, and K. Katayama, "Prolongation of QTc interval in patients with Parkinson's disease," *European Neurology*, vol. 37, no. 3, pp. 186–189, 1997.

[38] F. Ishizaki, T. Harada, H. Yoshinaga, T. Nakayama, Y. Yamamura, and S. Nakamura, "Prolonged QTc intervals in Parkinson's disease–relation to sudden death and autonomic dysfunction," *No to shinkei= Brain and nerve*, vol. 48, no. 5, pp. 443–448, 1996.

[39] M. C. Bakeberg, A. M. Gorecki, J. E. Kenna, A. Jefferson, M. Byrnes, S. Ghosh, M. K. Horne, S. McGregor, R. Stell, S. Walters *et al.*, "Elevated HDL levels linked to poorer cognitive ability in females with Parkinson's disease," *Frontiers in Aging Neuroscience*, vol. 13, p. 287, 2021.

[40] X. Huang, N. W. Sterling, G. Du, D. Sun, C. Stetter, L. Kong, Y. Zhu, J. Neighbors, M. M. Lewis, H. Chen *et al.*, "Brain cholesterol metabolism and Parkinson's disease," *Movement Disorders*, vol. 34, no. 3, pp. 386–395, 2019.

[41] O. Akbilgic, R. Kamaleswaran, A. Mohammed, G. W. Ross, K. Masaki, H. Petrovitch, C. M. Tanner, R. L. Davis, and S. M. Goldman, "Electrocardiographic changes predate Parkinson's disease onset," *Scientific Reports*, vol. 10, no. 1, pp. 1–6, 2020.

[42] A. A. Baumeister, "Is Attention-Deficit/Hyperactivity Disorder a Risk syndrome for Parkinson's disease?" *Harvard Review of Psychiatry*, vol. 29, no. 2, pp. 142–158, 2021.

[43] H.-C. Fan, Y.-K. Chang, J.-D. Tsai, K.-L. Chiang, J.-H. Shih, K.-Y. Yeh, K.-H. Ma, and I.-H. Li, "The association between Parkinson's disease and Attention-Deficit Hyperactivity Disorder," *Cell Transplantation*, vol. 29, p. 0963689720947416, 2020.

[44] S. Becker, M. J. Sharma, and B. L. Callahan, "ADHD and Neurodegenerative disease risk: A critical examination of the evidence," *Frontiers in Aging Neuroscience*, vol. 13, 2021.

[45] D. A. Kaminsky, D. G. Grosset, D. M. Kegler-Ebo, S. Cangiamilla, M. Klingler, P. Zhao, and C. Oh, "Natural history of lung function over one year in patients with Parkinson's disease," *Respiratory Medicine*, vol. 182, p. 106396, 2021.

[46] L. Marsh, "Depression and Parkinson's disease: current knowledge," *Current Neurology and Neuroscience Reports*, vol. 13, no. 12, pp. 1–9, 2013.

[47] F. M. Nilsson, L. V. Kessing, T. M. Sørensen, P. K. Andersen, and T. G. Bolwig, "Major depressive disorder in Parkinson's disease: a register-based study," *Acta Psychiatrica Scandinavica*, vol. 106, no. 3, pp. 202–211, 2002.

[48] A. M. Hemmerle, J. P. Herman, and K. B. Seroogy, "Stress, depression and Parkinson's disease," *Experimental Neurology*, vol. 233, no. 1, pp. 79–86, 2012.

[49] R. S. Wijeyekoon, D. Kronenberg-Versteeg, K. M. Scott, S. Hayat, J. L. Jones, M. R. Clatworthy, R. A. Floto, R. A. Barker, and C. H. Williams-Gray, "Monocyte function in Parkinson's disease and the impact of autologous serum on phagocytosis," *Frontiers in Neurology*, vol. 9, p. 870, 2018.

[50] K. Ando, K. Hamada, M. Shida, R. Ohkuma, Y. Kubota, A. Horiike, H. Matsui, T. Ishiguro, Y. Hirasawa, H. Ariizumi *et al.*, "A high number of PD-L1+ CD14+ monocytes in peripheral blood is correlated with shorter survival in patients receiving immune checkpoint inhibitors," *Cancer Immunology, Immunotherapy*, vol. 70, no. 2, pp. 337–348, 2021.

[51] H.-S. Lee, E. Lobbestael, S. Vermeire, J. Sabino, and I. Cleynen, "Inflammatory bowel disease and Parkinson's disease: common pathophysiological links," *Gut*, vol. 70, no. 2, pp. 408–417, 2021.

[52] T. Brudek, "Inflammatory bowel diseases and Parkinson's disease," *Journal of Parkinson's Disease*, vol. 9, no. s2, pp. S331–S344, 2019.

[53] M. K. Herrick and M. G. Tansey, "Is LRRK2 the missing link between inflammatory bowel disease and Parkinson's disease?" *npj Parkinson's Disease*, vol. 7, no. 1, pp. 1–7, 2021.

[54] Q. Deng, X. Zhou, J. Chen, M. Pan, H. Gao, J. Zhou, D. Wang, Q. Chen, X. Zhang, Q. Wang *et al.*, "Lower hemoglobin levels in patients with Parkinson's disease are associated with disease severity and iron metabolism," *Brain Research*, vol. 1655, pp. 145–151, 2017.

[55] R. D. Abbott, G. W. Ross, C. M. Tanner, J. K. Andersen, K. H. Masaki, B. L. Rodriguez, L. R. White, and H. Petrovitch, "Late-life hemoglobin and the incidence of Parkinson's disease," *Neurobiology of Aging*, vol. 33, no. 5, pp. 914–920, 2012.

[56] J. A. Santiago and J. A. Potashkin, "Blood transcriptomic meta-analysis identifies dysregulation of hemoglobin and iron metabolism in Parkinson's disease," *Frontiers in Aging Neuroscience*, vol. 9, p. 73, 2017.

[57] J. Freed and L. Chakrabarti, "Defining a role for hemoglobin in Parkinson's disease," *npj Parkinson's Disease*, vol. 2, no. 1, pp. 1–4, 2016.

[58] S. L. Rhodes and B. Ritz, "Genetics of iron regulation and the possible role of iron in Parkinson's disease," *Neurobiology of Disease*, vol. 32, no. 2, pp. 183–195, 2008.

[59] L. Shi, C. Huang, Q. Luo, E. Rogers, Y. Xia, W. Liu, W. Ma, W. Zeng, L. Gong, J. Fang *et al.*, "The association of iron and the pathologies of Parkinson's diseases in MPTP/MPP+-induced neuronal degeneration in non-human primates and in cell culture," *Frontiers in Aging Neuroscience*, vol. 11, p. 215, 2019.

[60] C. Wang, C. Zhou, T. Guo, P. Huang, X. Xu, and M. Zhang, "Association between cigarette smoking and Parkinson's disease: a neuroimaging study," *Therapeutic Advances in Neurological Disorders*, vol. 15, p. 17562864221092566, 2022.

[61] B. Ritz, P.-C. Lee, C. F. Lassen, and O. A. Arah, "Parkinson's disease and smoking revisited: ease of quitting is an early sign of the disease," *Neurology*, vol. 83, no. 16, pp. 1396–1402, 2014.

[62] F.-C. Yeh, H.-C. Chen, Y.-C. Chou, C.-L. Lin, C.-H. Kao, H.-Y. Lo, F.-C. Liu, and T.-Y. Yang, "Positive association of Parkinson's disease with ankylosing spondylitis: a nationwide population-based study," *Journal of Translational Medicine*, vol. 18, no. 1, pp. 1–8, 2020.

[63] C. R. Swanson, K. Li, T. L. Unger, M. D. Gallagher, V. M. Van Deerlin, P. Agarwal, J. Leverenz, J. Roberts, A. Samii, R. G. Gross *et al.*, "Lower plasma apolipoprotein A1 levels are found in Parkinson's disease and associate with apolipoprotein A1 genotype," *Movement Disorders*, vol. 30, no. 6, pp. 805–812, 2015.

[64] H. Y. Park, J. H. Lee, S. Y. Lee, D. S. Yu, K.-D. Han, Y. G. Park, and Y. B. Lee, "Risk for Parkinson's disease in patients with Behçet's disease: A nationwide population-based dynamic cohort study in Korea," *Journal of Parkinson's Disease*, vol. 9, no. 3, pp. 583–589, 2019.

[65] Y.-P. Huang, L.-S. Chen, M.-F. Yen, C.-Y. Fann, Y.-H. Chiu, H.-H. Chen, and S.-L. Pan, "Parkinson's disease is related to an increased risk of ischemic stroke—a population-based propensity score-matched follow-up study," *PLOS One*, vol. 8, no. 9, p. e68314, 2013.

[66] R. Caslake, K. S. Taylor, and C. E. Counsell, "Parkinson's disease misdiagnosed as stroke," *Case Reports*, vol. 2009, p. bcr0720080558, 2009.

[67] A. Marques, F. Dutheil, E. Durand, I. Rieu, A. Mulliez, M. L. Fantini, Y. Boirie, and F. Durif, "Glucose dysregulation in Parkinson's disease: Too much glucose or not enough insulin?" *Parkinsonism & Related Disorders*, vol. 55, pp. 122–127, 2018.

[68] R. Sandyk, "The relationship between diabetes mellitus and Parkinson's disease," *International Journal of Neuroscience*, vol. 69, no. 1-4, pp. 125–130, 1993.

[69] L.-L. Zhong, Y.-Q. Song, X.-Y. Tian, H. Cao, and K.-J. Ju, "Level of uric acid and uric acid/creatinine ratios in correlation with stage of Parkinson's disease," *Medicine*, vol. 97, no. 26, 2018.

[70] J.-J. Mo, L.-Y. Liu, W.-B. Peng, J. Rao, Z. Liu, and L.-L. Cui, "The effectiveness of creatine treatment for Parkinson's disease: an updated meta-analysis of randomized controlled trials," *BMC Neurology*, vol. 17, no. 1, pp. 1–9, 2017.

[71] D. A. Bosco, M. J. LaVoie, G. A. Petsko, and D. Ringe, "Proteostasis and movement disorders: Parkinson's disease and amyotrophic lateral sclerosis," *Cold Spring Harbor Perspectives in Biology*, vol. 3, no. 10, p. a007500, 2011.

[72] V. Arnao, A. Cinturino, S. Mastrilli, C. Buttà, C. Maida, A. Tuttolomondo, P. Aridon, and M. D'Amelio, "Impaired circadian heart rate variability in Parkinson's disease: a time-domain analysis in ambulatory setting," *BMC Neurology*, vol. 20, no. 1, pp. 1–5, 2020.

[73] A. Alonso, X. Huang, T. H. Mosley, G. Heiss, and H. Chen, "Heart rate variability and the risk of Parkinson's disease: a therosclerosis risk in communities study," *Annals of Neurology*, vol. 77, no. 5, pp. 877–883, 2015.

[74] G. Kenangil, B. Ari, F. Kaya, M. Demir, and F. Domac, "Red cell distribution width levels in Parkinson's disease patients," *Acta Neurologica Belgica*, vol. 120, no. 5, pp. 1147–1150, 2020.

[75] C. Fardell, K. Toren, L. Schioler, H. Nissbrandt, and M. Aberg, "High IQ in early adulthood is associated with Parkinson's disease," *Journal of Parkinson's Disease*, vol. 10, no. 4, pp. 1649–1656, 2020.

[76] X. Gao, K. C. Simon, J. Han, M. A. Schwarzschild, and A. Ascherio, "Genetic determinants of hair color and Parkinson's disease risk," *Annals of Neurology*, vol. 65, no. 1, pp. 76–82, 2009.

[77] A. Koçer, A. Yaman, E. Niftaliyev, H. Dürüyen, M. Eryılmaz, and E. Koçer, "Assessment of platelet indices in patients with neurodegenerative diseases: mean platelet volume was increased in patients with Parkinson's disease," *Current Gerontology and Geriatrics Research*, vol. 2013, 2013.

[78] J. Caplliure-Llopis, D. Escriv, E. Navarro-Illana, M. Benlloch, J. E. de la Rubia Orti, and C. Barrios, "Bone Quality in Patients with Parkinson's Disease Determined by Quantitative Ultrasound (QUS) of the Calcaneus: Influence of Sex Differences," *International Journal of Environmental Research and Public Health*, vol. 19, no. 5, p. 2804, 2022.

[79] G. S. Watson and J. B. Leverenz, "Profile of cognitive impairment in Parkinson's disease," *Brain Pathology*, vol. 20, no. 3, pp. 640–645, 2010.

[80] S. Cipriani, X. Chen, and M. A. Schwarzschild, "Urate: a novel biomarker of Parkinson's disease risk, diagnosis and prognosis," *Biomarkers in Medicine*, vol. 4, no. 5, pp. 701–712, 2010.

[81] M. Wen, B. Zhou, Y.-H. Chen, Z.-L. Ma, Y. Gou, C.-L. Zhang, W.-F. Yu, and L. Jiao, "Serum uric acid levels in patients with Parkinson's disease: A meta-analysis," *PlOS One*, vol. 12, no. 3, p. e0173731, 2017.

[82] C. T. Hong, Y. H. Huang, H. Y. Liu, H.-Y. Chiou, L. Chan, and L.-N. Chien, "Newly diagnosed anemia increases risk of Parkinson's disease: a population-based cohort study," *Scientific Reports*, vol. 6, no. 1, pp. 1–7, 2016.

[83] J. H. Kim, J. K. Oh, J. H. Wee, C. Y. Min, D. M. Yoo, and H. G. Choi, "The association between anemia and Parkinson's disease: a nested case-control study using a national health screening cohort," *Brain Sciences*, vol. 11, no. 5, p. 623, 2021.

[84] M. Fais, A. Dore, M. Galioto, G. Galleri, C. Crosio, and C. Iaccarino, "Parkinson's disease-related genes and lipid alteration," *International Journal of Molecular Sciences*, vol. 22, no. 14, p. 7630, 2021.

[85] A.-H. Ravn, J. P. Thyssen, and A. Egeberg, "Skin disorders in Parkinson's disease: potential biomarkers and risk factors," *Clinical, Cosmetic and Investigational Dermatology*, vol. 10, p. 87, 2017.

[86] A. Hassan, R. S. Kandel, R. Mishra, J. Gautam, A. Alaref, and N. Jahan, "Diabetes mellitus and Parkinson's disease: shared pathophysiological links and possible therapeutic implications," *Cureus*, vol. 12, no. 8, 2020.

[87] D. Sergi, J. Renaud, N. Simola, and M.-G. Martinoli, "Diabetes, a contemporary risk for Parkinson's disease: epidemiological and cellular evidences," *Frontiers in Aging Neuroscience*, vol. 11, p. 302, 2019.

[88] X. Huang, S. Y.-E. Ng, N. S.-Y. Chia, S. Acharyya, F. Setiawan, Z. Lu, Y. J. Tan, E. Ng, M.-C. Wen, A. S. Ng *et al.*, "Higher serum triglyceride levels are associated with Parkinson's disease mild cognitive impairment," *Movement Disorders: Official Journal of the Movement Disorder Society*, vol. 33, no. 12, pp. 1970–1971, 2018.

[89] M. R. H. Tehrani and M. Poursadeghfard, "Parkinson's disease accompanied by primary biliary cirrhosis: A case report," *Gastroenterology Nursing*, vol. 43, no. 2, pp. 196–198, 2020.

[90] V. A. Mosher, M. G. Swain, J. X. Pang, G. G. Kaplan, K. A. Sharkey, G. M. MacQueen, and B. G. Goodyear, "Primary biliary cholangitis alters functional connections of the brain's deep gray matter," *Clinical and Translational Gastroenterology*, vol. 8, no. 7, p. e107, 2017.

[91] M. Pajares, A. I Rojo, G. Manda, L. Boscá, and A. Cuadrado, "Inflammation in Parkinson's disease: mechanisms and therapeutic implications," *Cells*, vol. 9, no. 7, p. 1687, 2020.

[92] M. G. Tansey, R. L. Wallings, M. C. Houser, M. K. Herrick, C. E. Keating, and V. Joers, "Inflammation and immune dysfunction in Parkinson's disease," *Nature Reviews Immunology*, pp. 1–17, 2022.

[93] M. A. Moseng, J. C. Nix, and R. C. Page, "Biophysical consequences of even-plus syndrome mutations for the function of mortalin," *The Journal of Physical Chemistry B*, vol. 123, no. 16, pp. 3383–3396, 2019.
