# Supplementary material for: Assessing the Reproducibility of Machine-learning-based Biomarker Discovery in Parkinson's Disease
Source: arXiv:2304.03239 source file (2023-04-06)

**Supplementary Figures:** Venn diagrams of SNPs obtained by different approaches and same dataset. The diagrams below show the results of Autopsy, NINDS1, NINDS2 and Tier1 respectively. Approaches are identified by its number as in the main text: 0 – no integration.

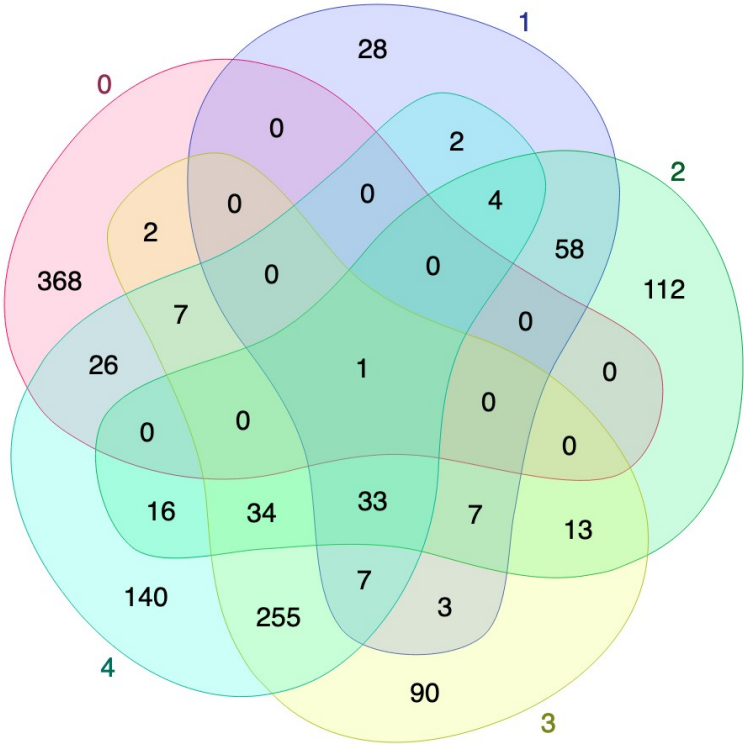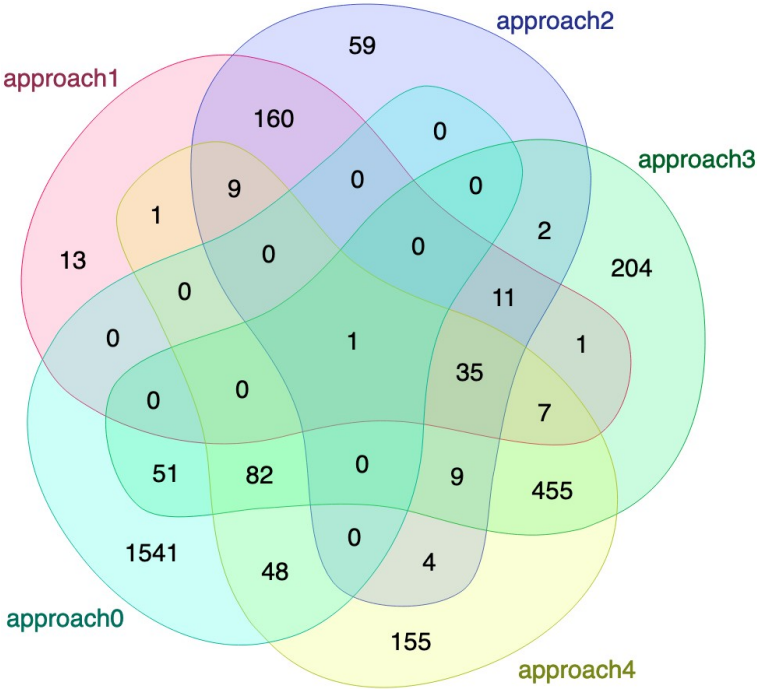

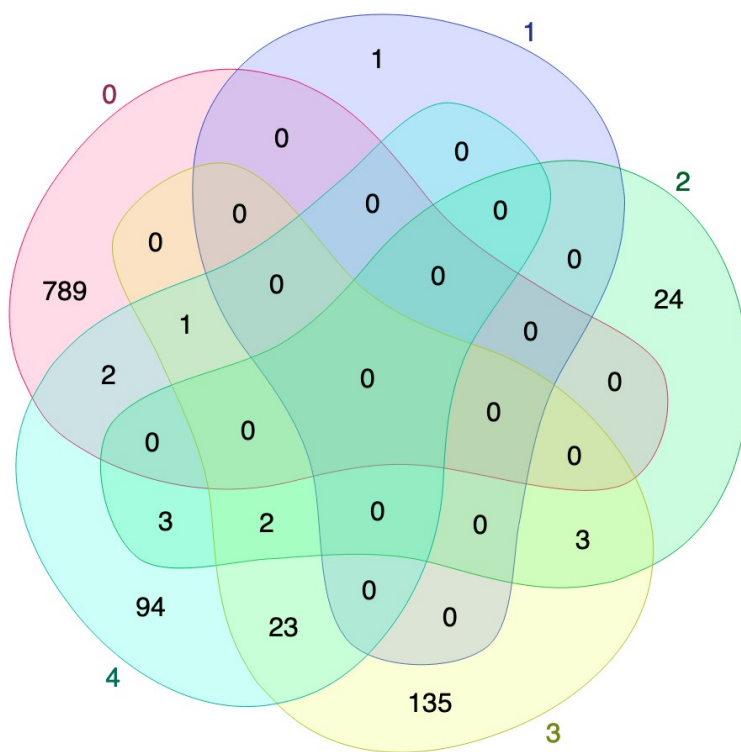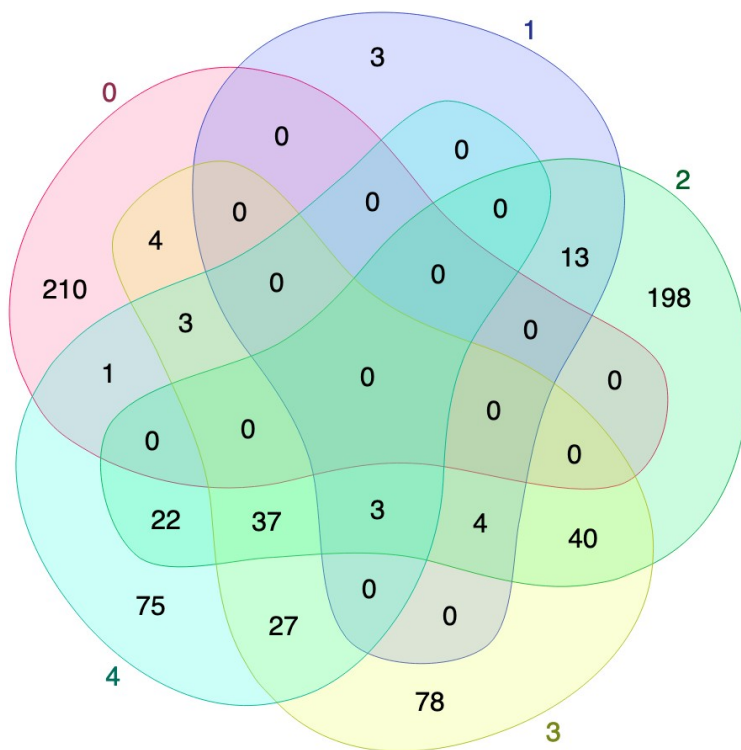

Supplement: Supplementary file 2 [file SupplementaryFigures.pdf]
